# Supplementary material for: Occamy: A Preemptive Buffer Management for On-chip Shared-memory Switches
Source: arXiv:2501.13570 source file (2025-01-23)
Supplement: Supplementary file 1 [file appendix.tex]

\clearpage
\appendix
\section*{Supplementary Material}
